# Supplementary material for: All-optical control of surface plasmons by second-harmonic generation
Source: arXiv:1801.05293 source file (2018-01-16)
Supplement: Supplementary file 1 [file SHG_coherent_SPP_SM.pdf]

# Supplemental Material: All-optical control of surface plasmons by second-harmonic generation

Sergio G. Rodrigo*

*Instituto de Ciencia de Materiales de Aragón and*
*Departamento de Física de la Materia Condensada,*
*CSIC-Universidad de Zaragoza, E-50009, Zaragoza, Spain and*
*Centro Universitario de la Defensa,*
*Ctra. de Huesca s/n, E-50090 Zaragoza, Spain*

(Dated: January 16, 2018)

*Electronic address: sergut@unizar.es

## I. SHG FROM A FLAT METAL SURFACE

We use the Finite-Difference Time-Domain (FDTD) method to compute induced polarization currents and optical near fields. In centrosymmetric materials, e.g. metals, Second Harmonic Generation (SHG) is electric-dipole forbidden in the bulk, so only the first high order leading terms (electric-quadrupole, magnetic-dipole...) contribute to SHG [1]. In addition, SH fields may generate at metal surfaces because inversion symmetry is broken [2–5]. The bulk contribution can not be neglected in flat metal surfaces [6] and the second-order polarization, $\mathbf{P}^{(\mathrm{SH})}$, would thus include both surface and bulk contributions. However, bulk contributions can be cast into a surfacelike model [4], an approach which is valid if nonlocal effects can be safely neleglected [7]. The second order polarization reads:

$$\begin{aligned} \mathbf{P}_n^{(\mathrm{SH})} &= \left[\chi^{(2)}_{nnn}|E_n^{(\mathrm{FH})}|^2 + \chi^{(2)}_{ntt}|E_t^{(\mathrm{FH})}|^2\right]\mathbf{n} \\ \mathbf{P}_t^{(\mathrm{SH})} &= 2\chi^{(2)}_{tnt}E_n^{(\mathrm{FH})}\mathbf{E}_t^{(\mathrm{FH})} \end{aligned} \qquad (1)$$

where $n$ and $t$ stand for normal and tangential to the surface respectively, and $\chi_{ijk}$ are the non-vanishing components of an effective second-order susceptibility tensor. The Fundamental Harmonic (FH) electric field is taken at the metal surface and from it $\mathbf{P}^{(\mathrm{SH})}$ is calculated at the same location.

To check the validity of our *homemade* SHG FDTD code that we have applied to metallic nanostructures in the manuscript, we calculated SHG from a flat gold-air interface illuminated by a Gaussian beam [8] in oblique incidence and compared it to analytical results [9]. The Gaussian beam has been implemented in FDTD within the the Total-Field Scattered-Field formulation [10]. The dielectric constant of gold is obtained from Ref. [11] instead from Ref. [12] (the one in the manuscript). Given the uncertainty in measuring $\chi^{(2)}$, which strongly depends on the quality of the metal surface (affected by grain size, roughness and presence of chemical byproducts), and that it usually differs from one sample to another, the nonlinear response of gold is assumed weakly dispersive within the frequency band of interest. We have taken for gold at all frequencies the (internal field) effective second-order susceptibility from Ref. [6], that is: $\chi^{(2)}_{nnn} = 250.0$, $\chi^{(2)}_{tnt} = 3.6$, and $\chi^{(2)}_{ntt} = 1.0$ in units of $3.27\ 10^{-15}$ cm/V. The last values are the same as the ones used in the manuscript. None of these choices do modify the main conclusions presented in the manuscript.

An example of SH fields simulated with FDTD is shown in Fig. 1. Panel (a) shows

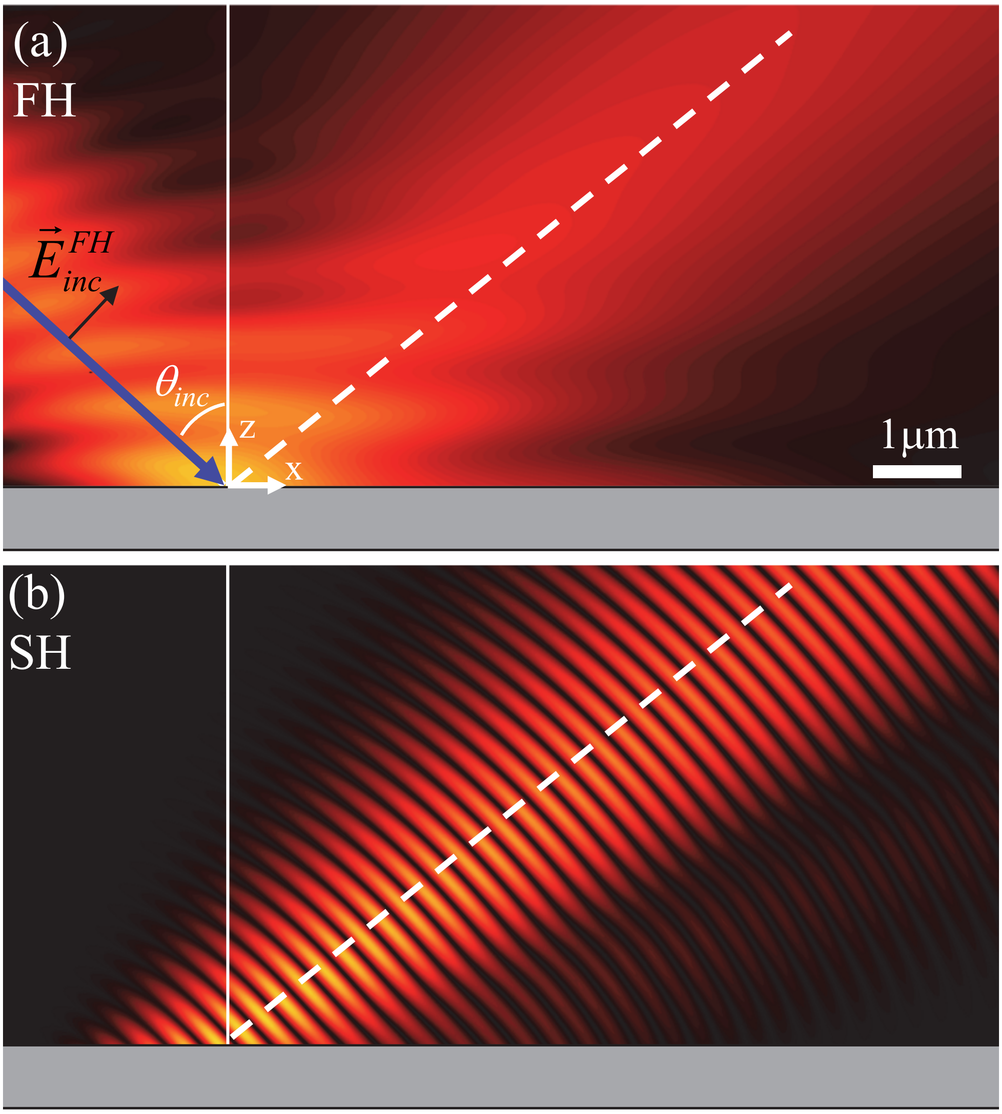


FIG. 1: Snapshots of the electric field amplitude from a gold-air interface obtained with FDTD when illuminated the surface by a linearly p-polarized Gaussian beam with central wavelength $\lambda_{FH} = 800$ nm at angle $\theta_{inc} = 45$ deg. (a) Fundamental Harmonic and (b) Second Harmonic.

a snapshot of the electric field amplitude from a gold-air interface when illuminated by a linearly p-polarized Gaussian beam with central wavelength $\lambda_{FH} = 800$ nm at angle $\theta_{inc} = 45$ deg. Panel (b) shows the corresponding SH field, which propagates from the metal surface at the same angle that of incidence of the FH due to momentum conservation.

We thus calculated the linear reflectance and nonlinear emission efficiency from electromagnetic (EM) fields obtained as those shown in Fig. 1, for different angles. Figure 2(a) shows linear reflection $R_p$ and $R_s$ for p-polarized and s-polarized incident Gaussian beams

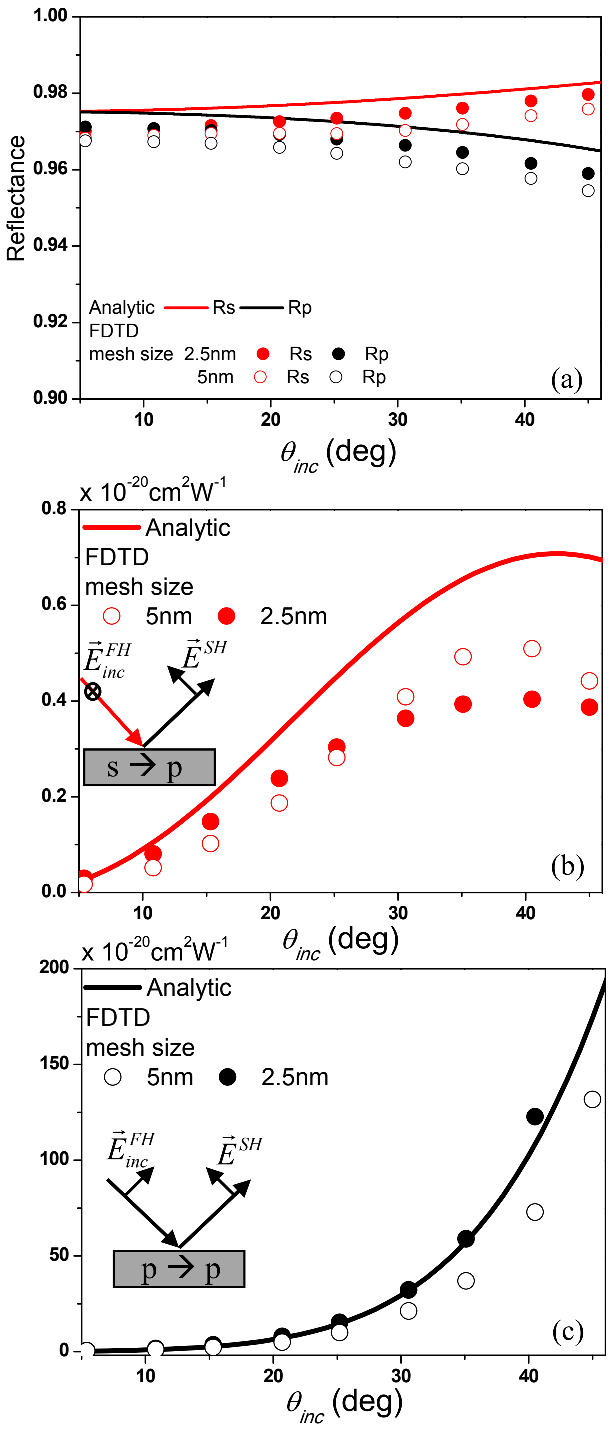


FIG. 2: (a) Linear reflection and (b)-(c) SHG emission efficiency for different polarizations, as a function of the incident angle $\theta_{inc}$ (defined in Fig. 1). Solid lines and symbols represent analytical and numerical results respectively. The analytical results were obtained for plane wave illumination while FDTD numerical results are for incident Gaussian beams and two different mesh sizes. The geometrical and materials parameters are the same that of Fig. 1.

respectively, as a function of the incident angle $\theta_{inc}$. Figure 2(b)-(c) shows the SHG emission efficiency for the *only* two possible incident to reflection combinations of light polarizations featuring SHG ($s \to p$ and $p \to p$, schematically represented in these panels). Solid lines and symbols are analytical and numerical results (two different FDTD mesh sizes), respectively. The geometrical and materials parameters are the same that of Fig. 1.

Overall the agreement is good between FDTD numerical calculations and analytical results in both linear and nonlinear regimes and improves with diminishing mesh size, as expected. A mesh size of 5 nm is enough to capture all aspects of SHG in flat metal surfaces, being the one used in the FDTD calculations of the manuscript. Note however that linear and nonlinear analytical expressions were obtained for a plane wave [9]. The use of a Gaussian beam makes the comparison with the analytical results more subtle. First, our nonlinear calculations are likely affected by the so-called Goos-Hanchen shift [13]. Second, $R_p$, $R_s$ and SHG emission efficiency must be defined as averaged quantities of the EM fields on the metal surface as follows.

For linear reflection:

$$R_{FH} = \left|\frac{\int S_z^{\text{reflected at FH}} dA}{\int S_z^{\text{incident at FH}} dA}\right| \tag{2}$$

, where $S_z$ is the z-component of Poynting's vector flux calculated at the gold surface ($z = 0$).

For SHG emission efficiency:

$$R_{SH} = A_{beam}\left|\frac{\int S_z^{\text{emitted at SH}} dA}{\left(\int S_z^{\text{incident at FH}} dA\right)^2}\right| \tag{3}$$

, where $A_{beam}$ is the area from which SH fields are generated and approximately coincides with the beam width. So defined, $R_{SH}$ is a quantity independent of the incident intensity and has units of $cm^2W^{-1}$.

Our FDTD implementation provides quantitative results for SHG in terms of intensity and properly takes into account the right components of the second order polarization [14].

## II. COHERENT CONTROL OF LATTICE DIFFRACTION ORDERS BY SHG

Radiative modes instead of evanescent and confined plasmonic modes can be controlled using our approach (see schematics Fig. 3(a)). In this case, our objective is to modify the relative intensity between different diffraction orders of the lattice.

At a fixed wavelength of light, only a finite number of k-vectors in a lattice are allowed to be radiative (diffraction orders) due to symmetry (Bloch's theorem). For example, in a slit array surrounded by air (the system investigated in this work) the dispersion relation is: $k_z = \sqrt{\frac{2\pi}{\lambda} - k_x^m}$, where $k_x^m = \frac{2\pi}{p}m$, $m = 0, \pm 1, ...$ (each diffraction order is labeled by a given value of $m$). The m-th diffraction order propagates at angle $\theta_m$ (see Fig. 3(c)) whenever the following expression is real valued: $sin(\theta_m) = \frac{m\lambda}{p}$.

In the example shown in Fig. 3, the period is chosen to be $p = 500$ nm ($p = 300$ nm in the manuscript - rest of parameters are equal), so for the signal beam ($\lambda = 450$ nm) apart from the specular diffraction order corresponding to $m = 0$, there are two diffraction orders allowed at angle $\theta_{m=\pm 1} \approx 64$ deg. In panel (b) we show the linear transmittance calculated for an infinite array of slits. Like in the slit array investigated in the manuscript the system is illuminated at normal incidence, the electric field polarized along the x-axis. In panel (c) we see the coherent control of the $m = \pm 1$ diffraction orders by changing the relative phase $\delta$ between signal and control beams. The sketch schematically shows the relative far-field intensity distribution of these diffraction orders expected at $\delta = 0.5$. We can distinguish the energy carried by the different diffracted orders with FDTD by projecting onto diffracted modes in each dielectric half space (for additional details see Ref. [15] and references therein).

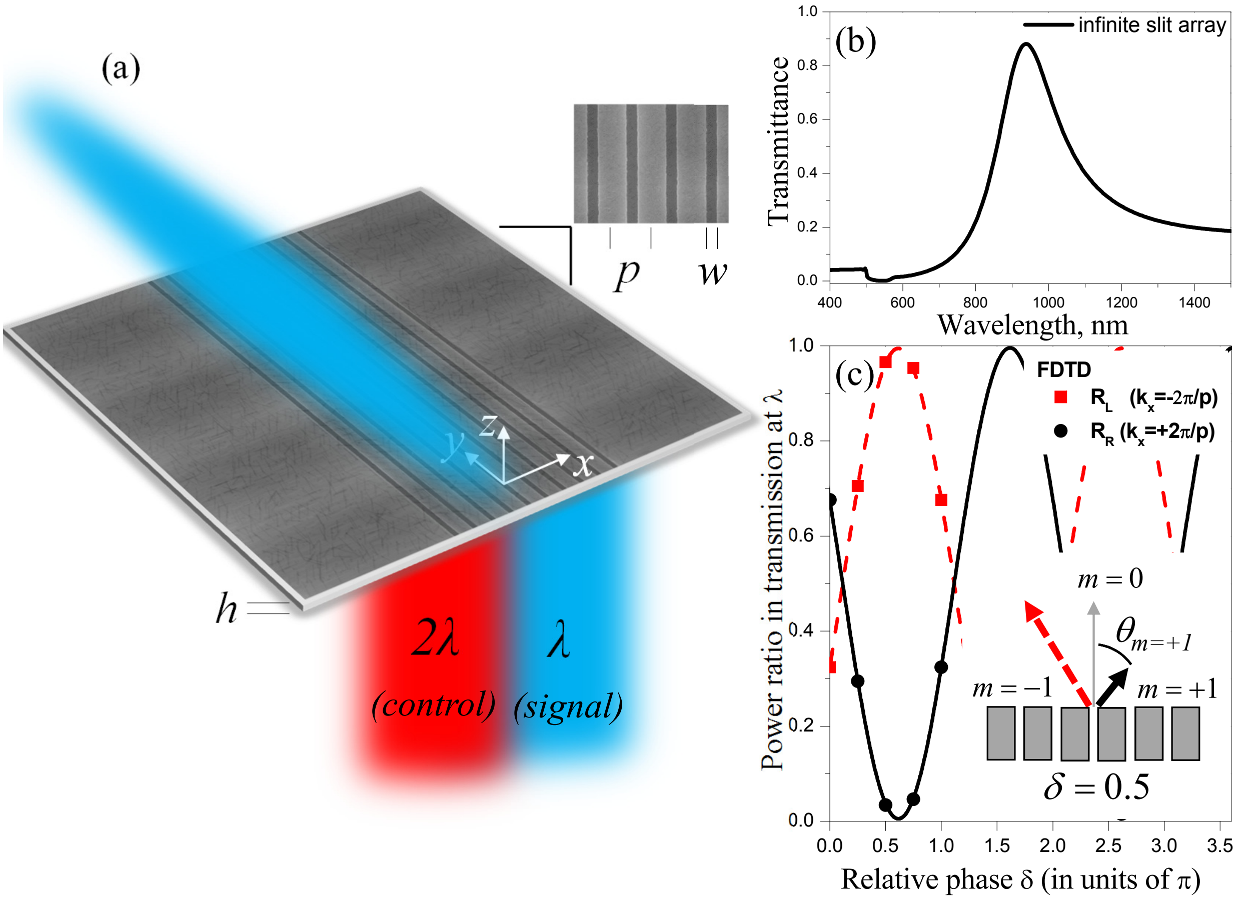


FIG. 3: (a) Schematics of active control of radiation by SHG. (b) Linear optical transmittance through an infinite array of slits. In linear and nonlinear calculations the system is illuminated at normal incidence, the electric field polarized along the x-axis. The geometrical parameters are $p = 500$ nm, $w = 100$ nm and $h = 300$ nm. The system is surrounded by air. (c) Control of the $m = \pm 1$ diffraction orders (angle $\approx 64$ deg) by the relative phase $\delta$ between signal and control beams at $\lambda = 450$ nm. The power ratio to the right (black) and to the left (red) are calculated with FDTD as a function of $\delta$ (symbols). The whole behavior is fitted to a sinusoidal function (solid lines). The sketch schematically shows the relative far-field intensity distribution between these diffraction orders at a fixed value of the relative phase, $\delta = 0.5$. For further details and definitions, see the manuscript.

## III. COHERENT CONTROL OF LONG-RANGE SPPS WITH A SINGLE METALLIC NANOWIRE ON TOP OF AN OPTICALLY THIN METAL FILM

To demonstrate coherent control of SPPs we have chosen a finite number of slits perforating an opaque metal film in the manuscript. We repeat here the same calculations but

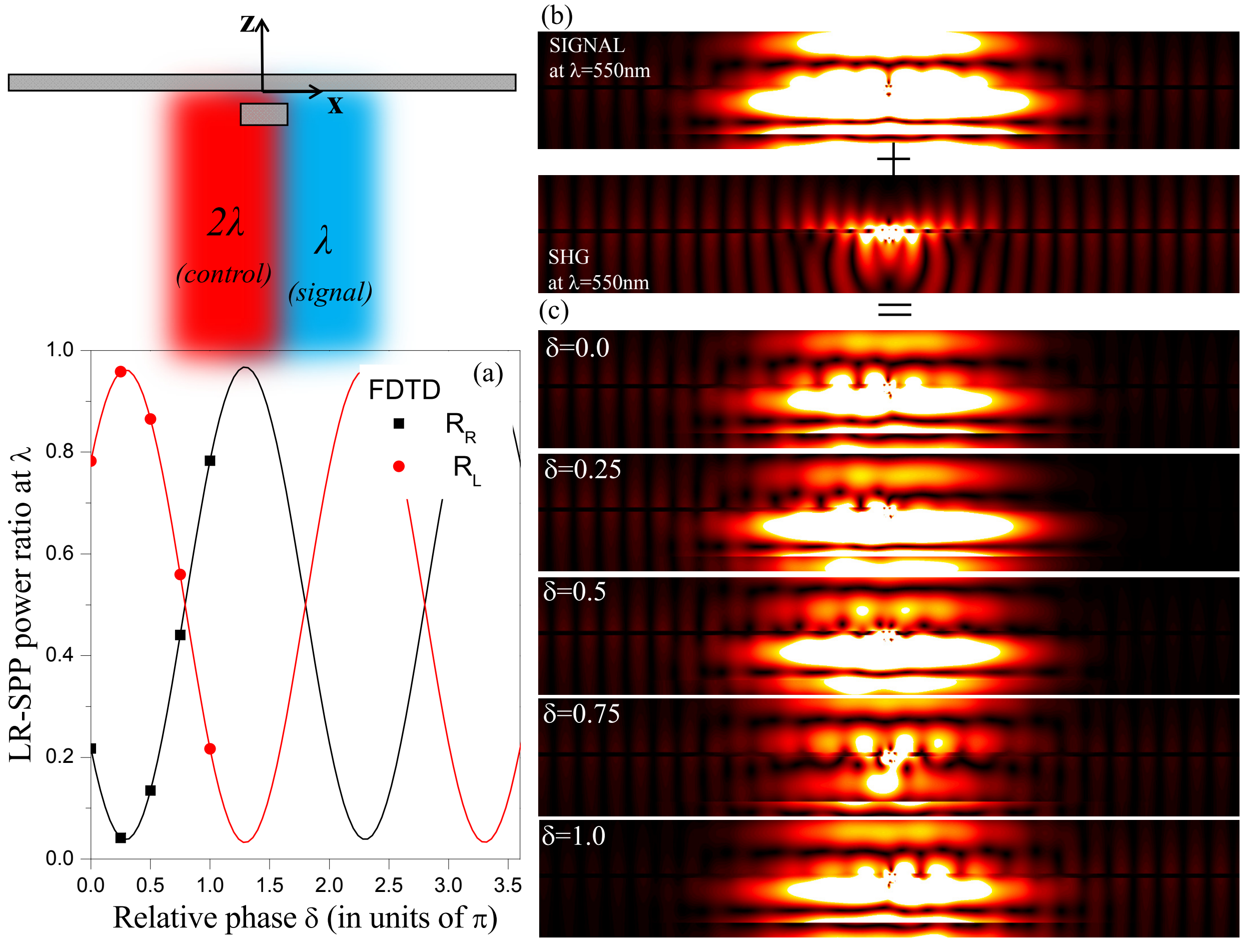


FIG. 4: (a) Coherent control of LR-SPP directionality by the relative phase $\delta$ between signal and control beams at $\lambda = 550$ nm. The power ratio to the right (black) and to the left (red) are calculated with FDTD as a function of $\delta$ (symbols). The whole behavior is fitted to a sinusoidal function (solid lines). Snapshots of the electric field amplitude: (b) top - scattered field from the signal beam at $\lambda = 550$ nm; bottom - the same at SH wavelength generated by the $2\lambda$ control beam, and (c) for values of $\delta$ calculated with FDTD [symbols in panel (a)], both beams are switched on. Map scale: red (maximum) and black (minimum). For further details and definitions, see the manuscript.

for a single gold nanowire separated 4 nm from a translucent metal film (the gold thickness of both nanowire and metal film is 30 nm and the horizontal width of the nanowire 100 nm). The non-metallic parts are air. The mesh size in FDTD calculations is 2 nm. Figure 4(b) shows snapshots of the electric field amplitude when the nanowire is solely illuminated by a signal beam (top) and the corresponding colour map for SHG (bottom).

Like in the slit array studied in the manuscript, there exist phase conditions for which surface plasmons on the metal film (here Long-Range SPPs) can be suppressed along one direction while they are simultaneously enhanced along the opposite direction, as demonstrated in Fig. 4(a) and Fig. 4(c). The first figure shows LR-SPP power ratios and the latter snapshots of the amplitude of the electric field in in a sequence of $\delta$ values taken from Fig. 4(a). The interference between the two terms can be tuned by adjusting the relative intensity and phase between them, thus $\mathbf{E}^{2\lambda}_{control} = \alpha \mathbf{E}^{\lambda}_{signal}$, where $\alpha = \alpha_0 \exp(i\delta\pi)$ and $\alpha_0 \sim 150$.

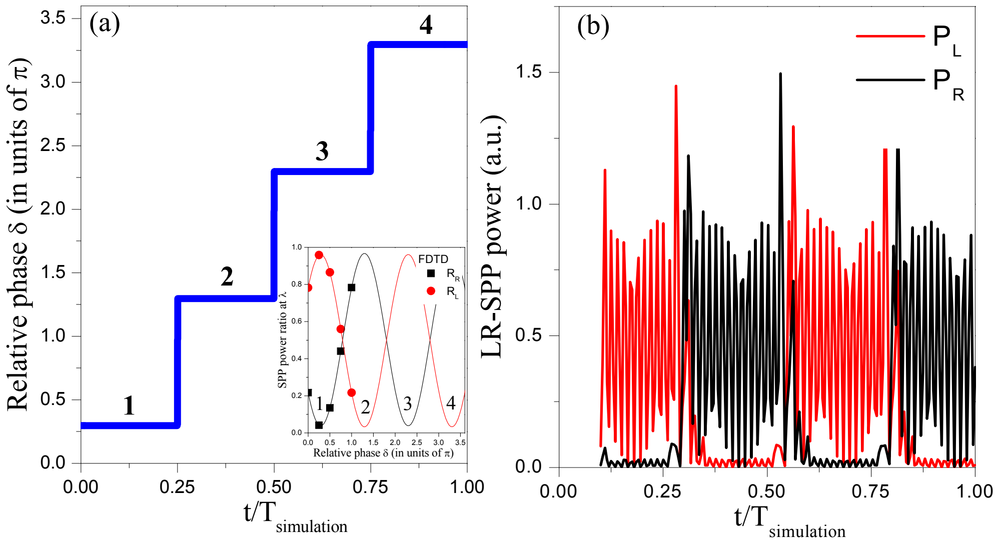


FIG. 5: Demonstration of dynamical control of Long-Range SPPs at $\lambda = 550$ nm. During a single FDTD simulation spanning $T_{\text{simulation}} \sim 0.4$ ps in time, the relative phase between signal and control beams is periodically changed as shown in (a). These values correspond to those labeled with integer numbers in the inset, which corresponds to an enhancement-suppression sequence of the Long-Range SPP current $P_L$ and $P_R$. (b) $P_L$ and $P_R$ powers are shown as a function of time. For definitions, see the manuscript.

Finally, we demonstrate in Fig. 5 dynamic control of Long-Range SPPs by changing the

relative phase between signal and control beams in time, like it is done in the manuscript for slit arrays and SPPs.

---


[1] N. Bloembergen, R. K. Chang, S. S. Jha, and C. H. Lee, Phys. Rev. **174**, 813 (1968).

[2] J. E. Sipe, V. C. Y. So, M. Fukui, and G. I. Stegeman, Phys. Rev. B **21**, 4389 (1980).

[3] M. Corvi and W. L. Schaich, Phys. Rev. B **33**, 3688 (1986).

[4] P. Guyot-Sionnest and Y. Shen, Phys. Rev. B **38**, 7985 (1988).

[5] V. Mizrahi and J. E. Sipe, J. Opt. Soc. Am. B **5**, 660 (1988).

[6] F. X. Wang, F. J. Rodríguez, W. M. Albers, R. Ahorinta, J. E. Sipe, and M. Kauranen, Phys. Rev. B **80**, 233402 (2009).

[7] C. Ciracì, E. Poutrina, M. Scalora, and D. R. Smith, Phys. Rev. B **86**, 115451 (2012).

[8] L. Novotny and B. Hecht, *Principles of Nano-Optics* (Cambridge University Press, Cambridge, 2012).

[9] K. A. O'Donnell and R. Torre, New J. Phys. **7**, 154 (2005).

[10] A. Taflove and S. C. Hagness, *Computational Electrodynamics: The Finite-Difference Time-Domain Method (Third edition)* (Artech House, Boston, 2005).

[11] S. G. Rodrigo, F. J. García-Vidal, and L. Martín-Moreno, Phys. Rev. B **77**, 075401 (2008).

[12] E. C. Hao, G. C. Schatz, R. C. Johnson, and J. T. Hupp, J. Chem. Phys. **117**, 5963 (2002).

[13] V. J. Yallapragada, A. V. Gopal, and G. S. Agarwal, Opt. Express **21**, 10878 (2013).

[14] K. N. Reddy, P. Y. Chen, A. I. Fernández-Domínguez, and Y. Sivan, J. Opt. Soc. Am. B **34**, 1824 (2017).

[15] S. G. Rodrigo, *Optical Properties of Nanostructured Metallic Systems: Studied with the Finite-Difference Time-Domain Method*, Springer Theses (Springer, 2011).
